# Supplementary material for: Significance-based community detection in weighted networks
Source: arXiv:1601.05630 source file (2017-10-23)
Supplement: Supplementary file 1 [file bw_Appendix_nontheory2.tex]

\begin{figure}
	\centering
	\makebox{
		\includegraphics[scale = 0.16]{Figures/CCME_applications/output_slpa_jan.png}
		\includegraphics[scale = 0.16]{Figures/CCME_applications/output_slpa_feb.png}
	}
	\makebox{
		\includegraphics[scale = 0.16]{Figures/CCME_applications/output_oslom_jan.png}
		\includegraphics[scale = 0.16]{Figures/CCME_applications/output_oslom_feb.png}
	}
	\makebox{
		\includegraphics[scale = 0.16]{Figures/CCME_applications/output_ccme_jan.png}
		\includegraphics[scale = 0.16]{Figures/CCME_applications/output_ccme_feb.png}
	}
	\caption{\label{fig:airports_jan-feb}SLPAw, OSLOM, and CCME results from January and Februrary 2015 U.S. airport networks. Maps created with $\mathtt{ggmap}$ \citep{ggmap}}
\end{figure}

\begin{figure}
	\centering
	\makebox{
		\includegraphics[scale = 0.16]{Figures/CCME_applications/output_slpa_mar.png}
		\includegraphics[scale = 0.16]{Figures/CCME_applications/output_slpa_apr.png}
	}
	\makebox{
		\includegraphics[scale = 0.16]{Figures/CCME_applications/output_oslom_mar.png}
		\includegraphics[scale = 0.16]{Figures/CCME_applications/output_oslom_apr.png}
	}
	\makebox{
		\includegraphics[scale = 0.16]{Figures/CCME_applications/output_ccme_mar.png}
		\includegraphics[scale = 0.16]{Figures/CCME_applications/output_ccme_apr.png}
	}
	\caption{\label{fig:airports_mar-apr}SLPAw, OSLOM, and CCME results from March and April 2015 U.S. airport networks. Maps created with $\mathtt{ggmap}$ \citep{ggmap}}
\end{figure}

\begin{figure}
	\centering
	\makebox{
		\includegraphics[scale = 0.16]{Figures/CCME_applications/output_slpa_may.png}
		\includegraphics[scale = 0.16]{Figures/CCME_applications/output_slpa_jul.png}
	}
	\makebox{
		\includegraphics[scale = 0.16]{Figures/CCME_applications/output_oslom_may.png}
		\includegraphics[scale = 0.16]{Figures/CCME_applications/output_oslom_jul.png}
	}
	\makebox{
		\includegraphics[scale = 0.16]{Figures/CCME_applications/output_ccme_may.png}
		\includegraphics[scale = 0.16]{Figures/CCME_applications/output_ccme_jul.png}
	}
	\caption{\label{fig:airports_may-jul}SLPAw, OSLOM, and CCME results from May and July U.S. airport networks. Maps created with $\mathtt{ggmap}$ \citep{ggmap}}
\end{figure}
%\FloatBarrier
%--------------------------------------------------------------------------------------------------------------------
